# Supplementary material for: Safe Reinforcement Learning via Probabilistic Shields
Source: arXiv:1807.06096 source file (2019-11-25)
Supplement: Supplementary file 1 [file appendix.tex]

\section{Appendix}
\subsection{Safety-Relevant Quotient MDP.}\label{safety_mdp}
Please find below an extended description and definition of the safety-relevant quotient MDP.

%We describe how to construct the safety-relevant (quotient) MDP we employ for safety analysis.
The construction of the MDP $\MdpInitR$ augments an arena by behavior models.
%  for adversaries. 
First, the \emph{states} $S=\Pos^{m+1} \times \{0,\hdots, m\}$ encode the positions for all agents and whose turn it is.
The \emph{actions} $\Act = \{ \act_0 \} \cup \Act_e$ determine the movements of the avatar and the adversaries:
% in the following way.
If agent $i$ moves next and its position is $(v,v',n)$ with $n > 0$, there is one unique action $\act_0$ at the corresponding state.
That action has a unique successor state where $n$ is decremented by one and $i$ incremented modulo $m$, \ie, agent $i+1$ will move next.
Thus, for $n>0$, there is no \textbf{decision} to be made.

If $n = 0$, the agent has to decide which edge $(v',v'')$ to select. 
This selection means that the position of agent $i$ is set to $(v',v'',d(v',v''))$ and again $i$ is incremented modulo $m$.
Edge selection has different types:
If $n=0$ and $i>0$ (an adversary moves next), there is a unique action $\act_0$ where the successor state is randomly determined according to the behavior $B_i$ for the current position of the adversary and the avatar. 
These transitions induce the only probabilistic choices in the MDP.
If $n = 0$ and $i=0$ (the avatar moves next), there is an action $\act_e$ reflecting every outgoing edge $e\in E$.
% and the distributions are based on the uncertainty maps.

\begin{definition}[Safety-relevant MDP]
	For an arena $(V,E,d)$ with agents $0,\ldots,m$, where agent $0$ is the avatar and agents $1,\ldots,m$ are adversaries, let $B_1,\hdots, B_m$ be adversary behaviors.
	The safety-relevant quotient MDP $\MdpInitR$ is given by $S=\Pos^{m+1} \times \{0,\hdots, m\}$, $\Act = \{ \act_0 \} \cup \Act_e$ with $\Act_e=\{ \act_e \mid e \in E \}$, and assuming $s=(\pos_0,\ldots,\pos_m,i)\in S$ with $\pos_i=(v,v',n)$, and $s'=(\pos_0',\ldots,\pos_m',(i+1)\modulo m)\in S$, $\mathcal{P}$ is given by 
%	\begin{align*}
%		\pmdp(s,\act)(s')=
		\begin{numcases}{\pmdp(s,\act)(s')=}
			1 		 & \text{ if }\ $i\geq 0, n>0,\act=\act_0, \pos_i'=(v,v',n-1)$\label{safeMDP_1}\\
%					 &\quad \text{and } i'=(i+1)\modulo m\\
			1 		 & \text{ if }\ $i = 0, n=0, \act=\act_e,\pos_i'=(v',v'',d(v',v''))$,\label{safeMDP_2}\\
			  		 & \quad \text{and }$(v',v'')=e\in E$\nonumber \\
			B(v,c)(v',v'') & \text{ if }\ $i > 0, n=0, \act=\act_0, \pos_i'=(v',v'',d(v',v''))$,\label{safeMDP_3}\\
					 & \quad $\pos_0=(u,u',n'), \text{ and }z_v(u)=c$\nonumber.
		\end{numcases}
%	\end{align*}
%	The reward function $r$ remains undefined.
\end{definition}

\subsection{Further Details on Shield Optimization}
Below is a third option towards addressing the tradeoff between safety and performance, as imposed by the shield.
To that end, we assume a measure of \emph{progress}, given by $\progress\colon S \rightarrow [0,1]$.

\emph{Side Constraints.}
Side constraints can be deduced and formulated in many fashions.
We propose the use of sets of actions, which we refer to as \emph{progress sets}.
Consider an MDP $\mdp$ where some states $T$ are reachable from a state $s$, and this reachability is desirable. 
For instance, \[ T_s = \{ s' \in S \mid \progress(s') > \progress(s) \}.\]
Assume that in $\shielded{\mdp}$, states in $T_s$ are not reachable anymore.
Thus, there is at least one action along every path from $s$ to $T$ in the original $\mdp$ that is blocked by the shield and prevents progress. 
We put these actions into a progress set.
Then, a side constraint to the shield computation states that \emph{from each progress set, one action needs to be allowed}. 
%
%\begin{example}
%Consider $\val{s}{\mdp} = \{ \act_1 \mapsto 0.4, \act_2 \mapsto 0.6 \}$ and $\val{s'}{\mdp} = \{ \act_3 \mapsto 0.1, \act_4 \mapsto 0.7 \}$.	
%Let $\{ \act_1, \act_3 \}$ be a progress set.
%\end{example}
%
Computing shields independently is thus possible, but might lead to suboptimal results.
In fact, we propose to do a form of regret minimization. We compute the regret for adding actions, and sum over all these actions. 
The following optimization problem describes the regret minimization, with variables $t_{\act} \in \{0,1\}$ for each $\act \in \Act$.
\begin{align*}
\text{minimize} \quad &  \sum_{s \in S} \sum_{\act \in \Act(s)}
  \Big(\delta \cdot \optval{s}{\mdp} - \val{s}{\mdp}(a)\Big) \cdot t_{\act} \\
\text{subject to} \quad & \sum_{\act \in X} t_{\act} \geq 1 \quad  \forall \text{progress sets } X
 %\forall s \in S \quad & \regret{s}{\mdp} = \sum_{\act \in \Act(s)}
  %\Big(\delta \cdot \optval{s}{\mdp} - \val{s}{\mdp}(a)\Big) \cdot t_{\act}
\end{align*}
The problem may be encoded as a mixed integer linear program~\cite{schrijver1998theory}.
% or an optimization modulo linear arithmetic \cite{}.

%Downside is that progress sets are qualitative, do not favor more progress progress.

%These progress sets are similar to \emph{fairness assumptions} \cite[Sect.~5.1.6]{BK08} in model checking, but in fairness assumptions, the idea is that from a set of actions, one action \emph{must} be taken.

\subsection{Further Experimental Results for PAC-MAN}
Figure~\ref{fig:appendixpacman} contains an additional plot for a smaller version of PAC-MAN. Table~\ref{tab:table1_appendix} contains additional rows for small versions of PAC-MAN.
\begin{figure*}[h]
	\centering
	\subfigure[Small PAC-MAN]
	{
	 \raisebox{0.75\height}{\includegraphics[scale=0.07,bb= 10 0 1900 510]{pics/vido_pacman_traps.png}}
	\label{fig:video_small_appendix}
	}
	\qquad
	\subfigure[Resulting Scores for small PAC-MAN]
	{
      \scalebox{0.85}{
	  \begin{tikzpicture}
      \begin{axis}[
        legend style={at={(0.97,0.45)},anchor=east},
        width=7cm,height=5cm,
        grid=major,
        ymax=1000,
        xlabel=Training Episodes,
        ylabel=Average Reward,
        xtick={0,40,80,120,160,200,240,280}
        ]
        \addplot[mark=*, blue, solid] table[x=episodes,y=woshield] {datasets/small.dat};
        \addlegendentry{Without Shield}

        \addplot[mark=square*, orange, densely dashed]  table[x=episodes,y=wshield]  {datasets/small.dat};
        \addlegendentry{With Shield}
      \end{axis}
      \end{tikzpicture}
      \label{fig:result_small}
	  }
    }
	\subfigure[Classic PAC-MAN]
	{
	 \raisebox{0.35\height}{\includegraphics[scale=0.14,bb= 10 0 1000 510]{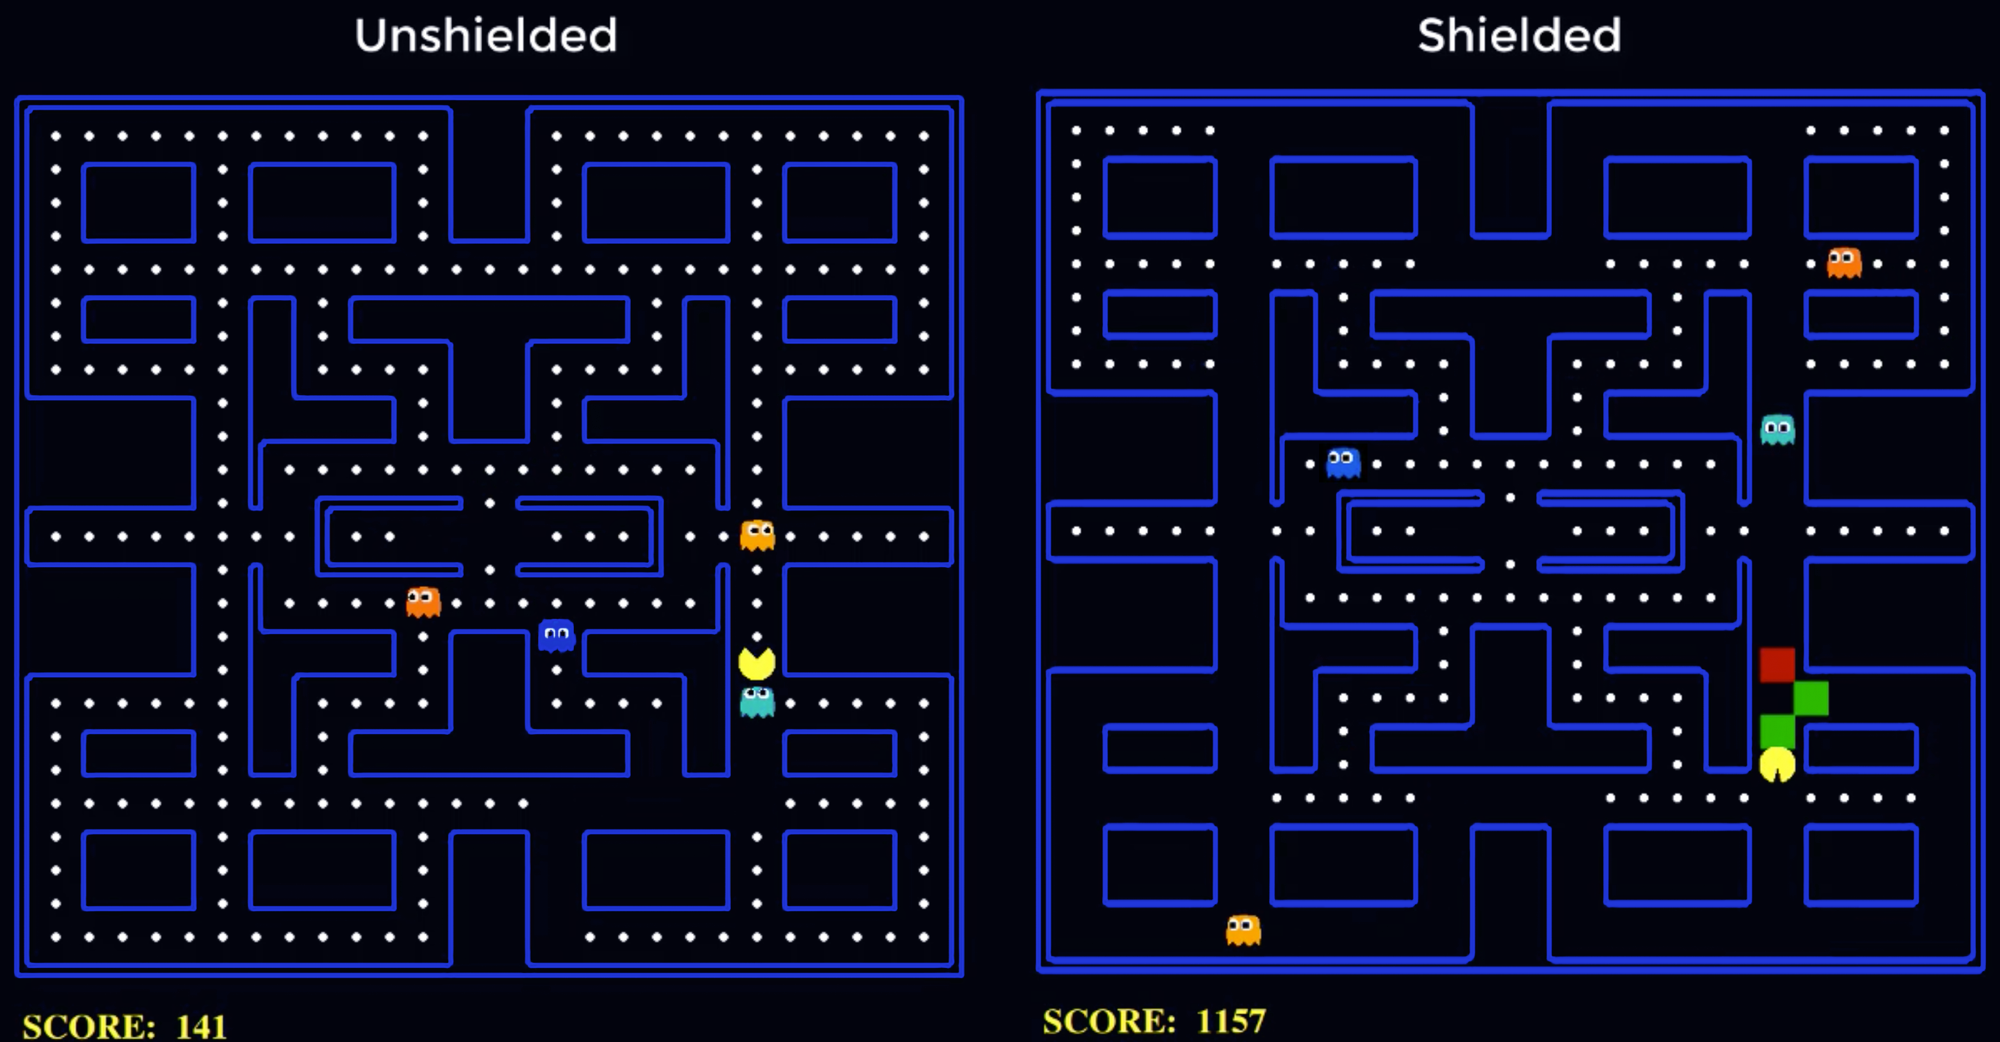}}
	\label{fig:video_classic_appendix}
	}
	\qquad
	\subfigure[Resulting Scores for Classic PAC-MAN]
	{
	  \scalebox{0.85}{
	  \begin{tikzpicture}
      \begin{axis}[
        legend pos=north west,
        width=7cm,height=5cm,
        grid=major,
        ymax=1000,
        xlabel=Training Episodes,
        ylabel=Average Reward,
        xtick={0,40,80,120,160,200,240,280}
        ]
        \addplot[mark=*, blue, solid] table[x=episodes,y=woshield] {datasets/classic.dat};
        \addlegendentry{Without Shield}

        \addplot[mark=square*, orange, densely dashed]  table[x=episodes,y=wshield]  {datasets/classic.dat};
        \addlegendentry{With Shield}
      \end{axis}
      \end{tikzpicture}
      \label{fig:result_classic_appendix}
	  }
	}	
	\caption{Scenarios and results for PAC-MAN}
	\label{fig:appendixpacman}
\end{figure*}

\begin{table*}[t]
\scriptsize
%  1 is the default, change whatever you need
\setlength{\tabcolsep}{0.45em} % for the horizontal padding
\centering
\caption{Experimental Results of Training}
\label{tab:table1_appendix}
\begin{tabular}{@{}|r|r|r|r|r|r|r|@{}}
\toprule
\multicolumn{1}{|l|}{\textbf{}}                                                         & \multicolumn{1}{l|}{\textbf{}}                                                                      & \multicolumn{1}{l|}{\textbf{}}
& \multicolumn{4}{l|}{\textbf{Total Results - Training}}                                                                                                                                                                                                                                                                                                                                   \\ \midrule
\multicolumn{1}{|c|}{\textbf{\begin{tabular}[c]{@{}c@{}}Size,\\ \#Ghosts\end{tabular}}} & \multicolumn{1}{c|}{\textbf{\begin{tabular}[c]{@{}c@{}}\#Model \\ Checking\end{tabular}}} & \multicolumn{1}{c|}{\textbf{time (s)}} & \multicolumn{1}{c|}{\textbf{\begin{tabular}[c]{@{}c@{}}Score\\  w/o Shield\end{tabular}}} & \multicolumn{1}{c|}{\textbf{\begin{tabular}[c]{@{}c@{}}Score with \\ Shield\end{tabular}}} & \multicolumn{1}{c|}{\textbf{\begin{tabular}[c]{@{}c@{}}Win Rate \\ w/o Shield\end{tabular}}} & \multicolumn{1}{c|}{\textbf{\begin{tabular}[c]{@{}c@{}}Win Rate \\ with Shield\end{tabular}}} \\ \midrule
5x5,1                                                                                   & 397                                                                                                 & 29                                      & 404,9                                                                                     & 505,9                                                                                        & 0,78                                                                                         & 0,89
\\ \midrule
6x5,1                                                                                   & 780                                                                                                 & 48                                      & -264                                                                                     & 391                                                                                        & 0,15                                                                                         & 0,85
\\ \midrule
9x7,1                                                                                   & 5912                                                                                                & 584                                   & -359,6                                                                                    & 535,3                                                                                     & 0,04                                                                                         & 0,84
\\ \midrule
17x6,2                                                                                  & 5841                                                                                                & 1072                                     & -195,6                                                                                    & 253,9                                                                                      & 0,04                                                                                         & 0,4
\\ \midrule
17x10,3                                                                                 & 51732                                                                                               & 3681                                   & -220,79                                                                                   & -40,52                                                                                     & 0,01                                                                                         & 0,07
\\ \midrule
27x25,4                                                                                 & 269426                                                                                              & 19941                                   & -129,25                                                                                   & 339,89                                                                                     & 0,00                                                                                          & 0,00
\\ \bottomrule
\end{tabular}
\end{table*}
\normalsize
